# Supplementary material for: First-Principles Study of the Fermi Surface Topology of CeCu$_{2}$Si$_{2}$
Source: arXiv:2412.18183 ancillary file (2025-12-30)
Supplement: Supplementary file 1 [file Ce122_SM.pdf]

# **Supplementary Material: First Principles Study of the Fermi Surface Topology of $\text{CeCu}_2\text{Si}_2$**

Roxanne M. Tutchton,<sup>1</sup> Jean-Pierre Julien,<sup>2</sup> Qimiao Si,<sup>3</sup> Jian-Xin Zhu,<sup>1</sup>

<sup>1</sup> *Theoretical Division, Los Alamos National Laboratory, Los Alamos, New Mexico 87545, USA*

<sup>2</sup> *Université Grenoble Alpes, CNRS, Institut NEEL, F-38042 Grenoble, France*

<sup>3</sup> *Department of Physics and Astronomy, Rice University, Houston, Texas 77005, USA*

## I. SUPPLEMENTARY THEORY

### A. Crystal Electric Field Derivation

Here we examine the Crystal Electric Field (CEF) that lifts up the degenerate  $j = 5/2$   $f$ -electron orbital subshell for the Cerium atom in a BCT environment of, primarily, 8 silicon atoms (approximated as point charges) in the compound  $CeSi_2Cu_2$ . These neighboring charges, located at  $\vec{a}_i = (a, \theta_i, \phi_i)$  (in spherical coordinates), produce an additional electrostatic potential  $V_{CF}$  on the Cerium  $4f$  electron of elementary charge  $q_0$  located at  $\vec{r} = (r, \theta, \phi)$ :

$$V_{CF}(\vec{r}) = \sum_{i=1}^N \frac{1}{4\pi\epsilon_0} \frac{q_0 Q_i}{|\vec{r} - \vec{a}_i|}. \quad (1)$$

This potential is treated as a perturbation. For degenerate levels, we write the matrix of this perturbation in the basis of degenerate states. As there is only one  $4f$  electron in Cerium ( $Z=58$ ), we are concerned with the 6 degenerate states of the  $j = 5/2$  subshell where the total angular momentum,  $\vec{J} = \vec{L} + \vec{S}$ , is adapted in presence of spin orbit coupling (SOC) and SOC splitting between the  $j = 5/2$  and  $j = 7/2$  (unoccupied) states, which is known to be on the order of 80meV. Expanding  $\frac{1}{|\vec{r} - \vec{a}_i|}$  in spherical harmonics, using Clebsch-Gordon coefficients (CG) to transform from the  $|lm_l\rangle$  basis to the  $|jm_j\rangle$  basis, and subsequent selection rules on products of spherical harmonics, we end up, apart from a negligible rigid shift on the diagonal (which would not lift the degeneracy) with the  $6 \times 6$  CEF potential matrix to be diagonalized. This matrix has the structure, ranging from state  $|j = \frac{5}{2}, m_j = -\frac{5}{2}\rangle$  to  $|j = \frac{5}{2}, m_j = +\frac{5}{2}\rangle$ :

$$[V_{CF}]_{5/2} = \begin{pmatrix} A & 0 & 0 & 0 & C & 0 \\ 0 & B & 0 & 0 & 0 & C \\ 0 & 0 & D & 0 & 0 & 0 \\ 0 & 0 & 0 & D & 0 & 0 \\ C & 0 & 0 & 0 & B & 0 \\ 0 & C & 0 & 0 & 0 & A \end{pmatrix} \quad (2)$$

This matrix can be split into two identical  $2 \times 2$  matrices expressed in terms of the states  $|j = \frac{5}{2}, m_j = \pm\frac{5}{2}\rangle$  and  $|j = \frac{5}{2}, m_j = \mp\frac{3}{2}\rangle$  as

$$\begin{pmatrix} A & C \\ C & B \end{pmatrix} \quad (3)$$

with eigenvalues  $\frac{A+B}{2} \pm \sqrt{(\frac{A-B}{2})^2 + C^2}$  and eigenstates

$$\alpha \left| \frac{5}{2}, \pm \frac{5}{2} \right\rangle + \sqrt{1 - \alpha^2} \left| \frac{5}{2}, \mp \frac{3}{2} \right\rangle \quad (4)$$

$$\sqrt{1 - \alpha^2} \left| \frac{5}{2}, \pm \frac{5}{2} \right\rangle - \alpha \left| \frac{5}{2}, \mp \frac{3}{2} \right\rangle \quad (5)$$

$$(6)$$

There are also two uncoupled, already diagonal, big matrices,  $[V_{CF}]_{5/2}$ , with degenerate states  $|j = \frac{5}{2}, m_j = \pm \frac{1}{2}\rangle$ .

For the direction of the Ce-Si bond, we use an angle  $\theta_0 = \frac{3\pi}{8}$  with a relative error of 0.02% compared to the real angle in the structure. This allows for the analytical expressions of matrix elements to be obtained as follows;

$$A = \frac{6\sqrt{2}-4}{7}I_2 + \frac{9-10\sqrt{2}}{168}I_4$$

$$B = -\frac{6\sqrt{2}-4}{35}I_2 - \frac{9-10\sqrt{2}}{56}I_4$$

$$C = \frac{(2\sqrt{2}-3)\sqrt{5}}{24}I_4$$

$$D = \frac{16-24\sqrt{2}}{35}I_2 + \frac{9-10\sqrt{2}}{84}I_4$$

The parameters  $[\frac{\langle r^k \rangle}{a^{k+1}}] \equiv I_k$  (k=2,4) govern all the physics of the CEF splitting and are expressed in term of the interatomic distance Ce-Si  $a$ , the charge  $Q$  of each silicon atom, a constant  $e = \frac{q_0}{4\pi\epsilon_0}$ , and an integral over the radial Ce 4f wave function

$$\langle r^k \rangle = \int r^k |R_{4f}(r)|^2 dr. \quad (7)$$

The ordering in energy of eigenvalues is directly related to the sign of the  $I_k$ 's, which can reverse the ordering. By way of electronic structure calculations, the charge  $Q$  of silicon in this compound is known to be positive and the elementary charge  $q_0$  is negative, therefore the overall sign of  $I_k$ 's is negative, giving a negative sign for the lowest eigenvalue. The lowest energy states (ground state) are the doublet of  $|\Gamma_7^{(1)} \pm\rangle$  which turn out to be:

$$|\Gamma_7^{(1)} \pm\rangle = \alpha \left| \frac{5}{2}, \pm \frac{5}{2} \right\rangle + \sqrt{1 - \alpha^2} \left| \frac{5}{2}, \mp \frac{3}{2} \right\rangle \quad (8)$$

where the value of  $\alpha$  is negative. Then the  $|\Gamma_7^{(2)}\pm\rangle$  doublet,

$$|\Gamma_7^{(2)}\pm\rangle = \sqrt{1-\alpha^2} \left| \frac{5}{2}, \pm\frac{5}{2} \right\rangle + |\alpha| \left| \frac{5}{2}, \mp\frac{3}{2} \right\rangle, \quad (9)$$

gives the first excited states, with the energy gap between this doublet and the ground state doublet, experimentally known to be of the order of 30meV. Finally, the highest states are given by the doublet

$$|\Gamma_6\pm\rangle = \left| \frac{5}{2}, \pm\frac{1}{2} \right\rangle. \quad (10)$$

As a consequence of Kramers theorem, each eigenstate has the same energy as its time reversal state, leading to the obtained doublets. Note that when we fit the  $I_k$ 's to reproduce the experimental gap, we always obtain this energy ordering, *i.e.*  $|\Gamma_6\pm\rangle$  is higher in energy than the first excited states  $|\Gamma_7^{(2)}\pm\rangle$ . This is in slight disagreement with the results of Rueff *et al.*[1].

To complete our analysis, we performed two other calculations to verify our conclusions about the nature and symmetry of the ground state and the first excited states:

1) Since SOC is known to be on the order of 80 meV and the CFS is, experimentally, about 30 meV, the application of perturbation theory needs to be approached with caution. To validate this approximation, we wrote the entire CEF matrix on the full  $l = 3$  space split in 5/2 and 7/2 subspaces. There are indeed non-zero off diagonal subblocks 5/2-7/2, but we do not change the physical conclusion as a result.  $|\Gamma_7^{(1)}\pm\rangle$  and  $|\Gamma_7^{(2)}\pm\rangle$  are still the ground state and the first excited state respectively with the small admixture of the  $j = 7/2$  states with same  $m_j = \pm 5/2, \mp 3/2$ . The perturbation approximation of the  $j = 5/2$  states is therefore validated.

2) The Ce atom has the second shell of negatively charged Cu atoms with an interatomic distance Ce-Cu  $a' = 3.22 \text{ \AA}$ , just slightly bigger than the interatomic distance Ce-Si  $a = 3.13 \text{ \AA}$ . We checked the effect of including this second shell, and again we saw that it does not change the main physical conclusion about  $|\Gamma_7^{(1)}\pm\rangle$  and  $|\Gamma_7^{(2)}\pm\rangle$ .

## II. SUPPLEMENTARY METHODS: DMFT CALCULATION

As in the case of the GGA+GWA method described in the main text (section 5.1), this method uses the FP-LAPW implementation of WIEN2k[2] as its basis. The DMFT calculation implements

a strong-coupling version of the continuous-time quantum Monte-Carlo (CT-QMC) method[3–5] in order to explicitly consider the on-site Coulomb interactions. In order to compare the DMFT results to those of the other methods, for which  $T=0$  K, the Fermi surface data was extrapolated from the  $T=0.01$  eV calculation where the electronic self-energies’ sensitivity to temperature is negligible. The Fermi energy was then shifted to maintain electron and hole occupations in each band consistent with  $T \rightarrow 0$  eV as dictated by the Fermi-Dirac distribution. The calculation results are discussed below and shown in FIG. S10.

### III. SUPPLEMENTARY RESULTS

The following discussion describes the results of our exploration of the CFS and electronic correlation effects on  $\text{CeCu}_2\text{Si}_2$ . The electronic ground state was calculated under several conditions (all including SOC in a non-collinear paramagnetic configuration): (1) Using the GWA with a PBE-GGA exchange correlation functional[6], (2) with electron-electron correlations, (3) With electron-electron correlations and CFS. The band dispersion, DOS, and Fermi surfaces have been documented for each case.

#### A. Electronic Structure

The electronic band dispersion and DOS calculated for  $U = 0$  are given in FIG.S1 (a) and (c) respectively. The three Fermi surface sheets are shown in FIG.S1 (b) in order of descending band number,  $b_n$ , from top to bottom. These results are in close agreement with those calculated in the early 1990’s by Harima *et al.*[7, 8]. The path through the first Brillouin zone (BZ) is shown in FIG. S2. Red lines are interposed on the Fermi surfaces in FIG.S1 (b) to indicate the cross sections related to the dHvA extremal frequencies for an external  $\mathbf{B}$  field parallel to the z-axis. The dHvA results for the Fermi surface are given in Table S2, which shows the results when CFS is included and when it is neglected. For small vales of  $U$ , the impact of CFS on the Fermi surface topology is minimal, and for  $U = 0$ eV it is negligible. Table S1 similarly shows the comparison of the quasiparticle weights,  $Z$ , of calculations with and without CFS. Here the difference is more significant do to the splitting of the  $j = 5/2$  orbital into  $\Gamma_7^{(1)}$ ,  $\Gamma_7^{(2)}$ , and  $\Gamma_6$  doublets.

In order to better understand the impact of the CFS in  $\text{CeCu}_2\text{Si}_2$  along with the interconnected effect of elctronic correlations, the band dispersions and densities of state for values of  $U$  from

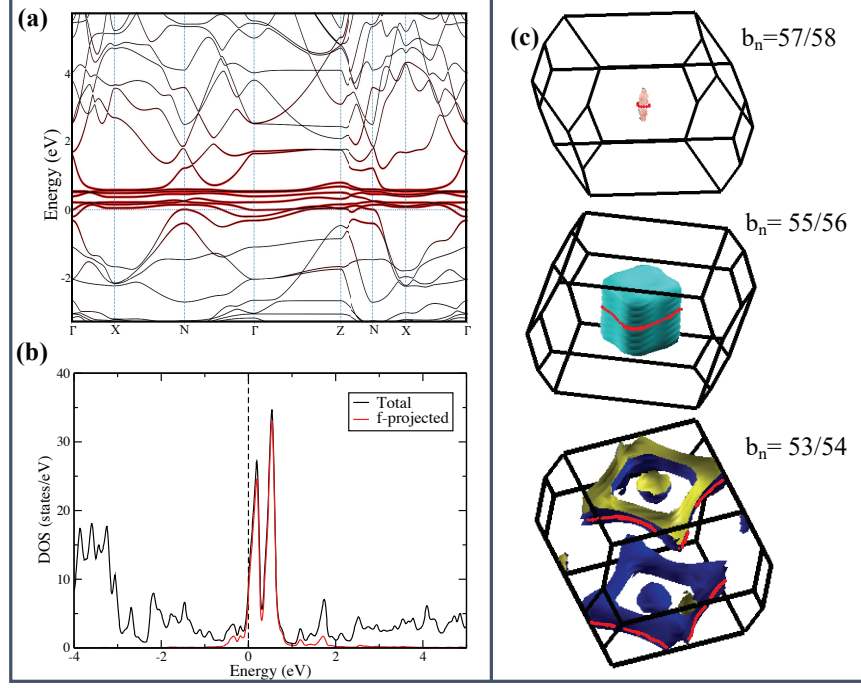

FIG. S1. **The electronic ground state calculation** for  $\text{CeCu}_2\text{Si}_2$  calculated using the GWA in the generalized gradient approximation (GGA) without electronic correlations. We include (a) the electronic band dispersion with black lines representing the total eigenenergy bands and red lines indicating the  $f$ -electron contribution, b) the Fermi surface sheets for degenerate bands 53 through 58, where each band is doubly degenerate due to the SOC, (c) the electron density of states (DOS) where the black line indicates the total DOS and the red the projected  $f$ -electron DOS. The high symmetry path through the BZ is shown in FIG. S2.

1 to 6 eV are shown in FIG. S3 and FIG. S4 respectively, with no CFS effects included in the GWA calculations. FIG. S5 and FIG. S6 show the calculations with CFS taken into account within the GWA. Given these results along with the data in Tables S1 and S2, the effect of CFS in the renormalized electronic structure are significant.

The band dispersions in FIG. S3, for example, show little evolution until  $U = 4\text{eV}$  (FIG. S3(d)), where a broadening of the bands around the Fermi energy starts to emerge and grow incrementally up to  $U = 6\text{eV}$ . This is confirmed by the corresponding DOS (FIG. S4) in which there are two peaks dominated by the localized  $f$ -electron orbital subshells ( $j = 5/2$  and  $j = 7/2$ ) from the Ce atom. These peaks remain close together ( $\lesssim 1\text{eV}$ ) until  $U = 4\text{eV}$ , where they start to separate slightly. This continues up to  $U = 6\text{eV}$  as the  $j = 5/2$  peak grows taller and narrower, becoming more delta-like, as  $U$  increases. Conversely, the  $j = 7/2$  peak appears at a higher energy while

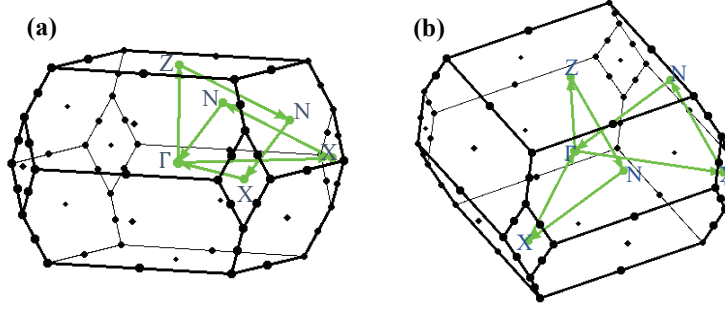

FIG. S2. **The high symmetry path through the first Brillouin zone** used for the band structure calculations from  $\Gamma \rightarrow L \rightarrow W \rightarrow X \rightarrow \Gamma$ . (a) and (b) show two different perspectives of the same path.

becoming shorter and wider as  $U$  increases. This is consistent with expected SOC splitting in a strongly coupled system[9].

Alternatively, with the CFS taken into account within the GWA, the band dispersions for increasing  $U$  are shown in FIG. S5. Once again there is little change until  $U = 4\text{eV}$  (FIG. S5(d)), then the impact of increasing  $U$  is significant at  $U = 5\text{eV}$  and  $U = 6\text{eV}$ . At  $U = 5\text{eV}$  (FIG. S5(e)) the  $f$ -electron bands spread out above the Fermi energy, and at  $U = 6\text{eV}$  the  $f$ -electron bands split with some collapsing to a nearly flat band at the Fermi energy and the rest localized around  $4\text{eV}$  above the Fermi energy. The DOS in FIG. S6 give a clearer picture of the evolution on the electron occupation. As with the DOS when the CFS is absent, there are two peaks near the Fermi energy dominated by the  $f$ -electron. As  $U$  increases the peaks separate (as they do in the absence of CFS effects), changing slightly until  $U = 5\text{eV}$  where the two peaks become three. This is consistent with the lifting of the Ce  $j = 5/2$  electrons do to CFS (see main text FIG.1).

Between  $U = 5\text{eV}$  and  $U = 6\text{eV}$  the change is more dramatic as a single, delta-like peak is left at the Fermi energy and the rest of the  $f$ -electrons are shifted up in energy and spread around  $4\text{eV}$ . Once again this is consistent with a splitting of the metallic  $j = 5/2$  and the insulating  $j = 7/2$  electrons. Here it is clear that the additional presence of CFS splitting is significant to the overall orbital structure. The relatively sudden evolution between  $U = 5$  and  $6\text{eV}$  in the presence of CFS was further explored in order to thoroughly capture the interconnected behavior between the electron correlation strength and the crystal field. The results of a calculation at  $U = 5.1\text{eV}$  are given in FIG. S7 and discussed in the main text. This slight increase in the Coulomb interaction strength (from 5 to  $5.1\text{eV}$ ) results in a barely perceptible change in the band dispersion, but the DOS does appear to shift to a stage that is recognizably between  $U = 5$  and  $6\text{eV}$  with a sharp peak

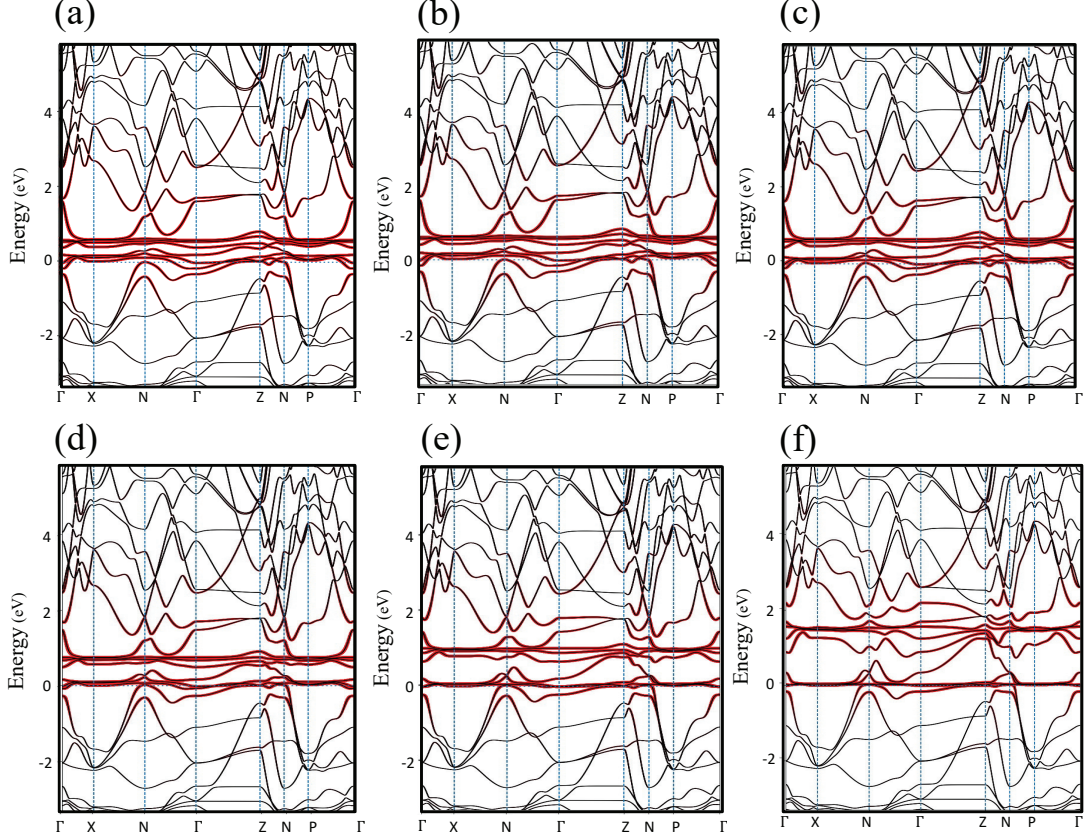

FIG. S3. **The electronic structure** for  $\text{CeCu}_2\text{Si}_2$  calculated using the GWA without CFS for increasing values of  $U$ : (a) 1eV, (b) 2eV, (c) 3eV, (d) 4eV, (e) 5eV, to (f) 6eV. The Hund parameter is  $J = 0.7\text{eV}$  for each calculation. The qualitative appearance of the band dispersions is relatively unchanged until  $U$  reaches a value of  $\sim 4\text{--}5\text{eV}$ , at which point the  $f$ -electron bands (indicated in red) begin to spread out around the Fermi energy. This spreading becomes slightly more pronounced at  $U = 6\text{eV}$ . This corresponds to the separation of the  $j = 5/2$  and  $j = 7/2$   $f$ -electron orbital subshells (see FIG. S4(f)).

at the Fermi energy and a more disperse arrangement of the higher energy quasiparticle states.

### 1. Quasiparticle weights

Here we include further detail on the quasiparticle weight analysis discussed in the main text. The eigenvalues of the  $4f$  quasiparticle matrix,  $Z$ , given in Table S1 along with the corresponding orbital occupations,  $n$  for  $U = 0$  through 6eV. These are derived from the ‘‘Gutzwiller self-energy’’

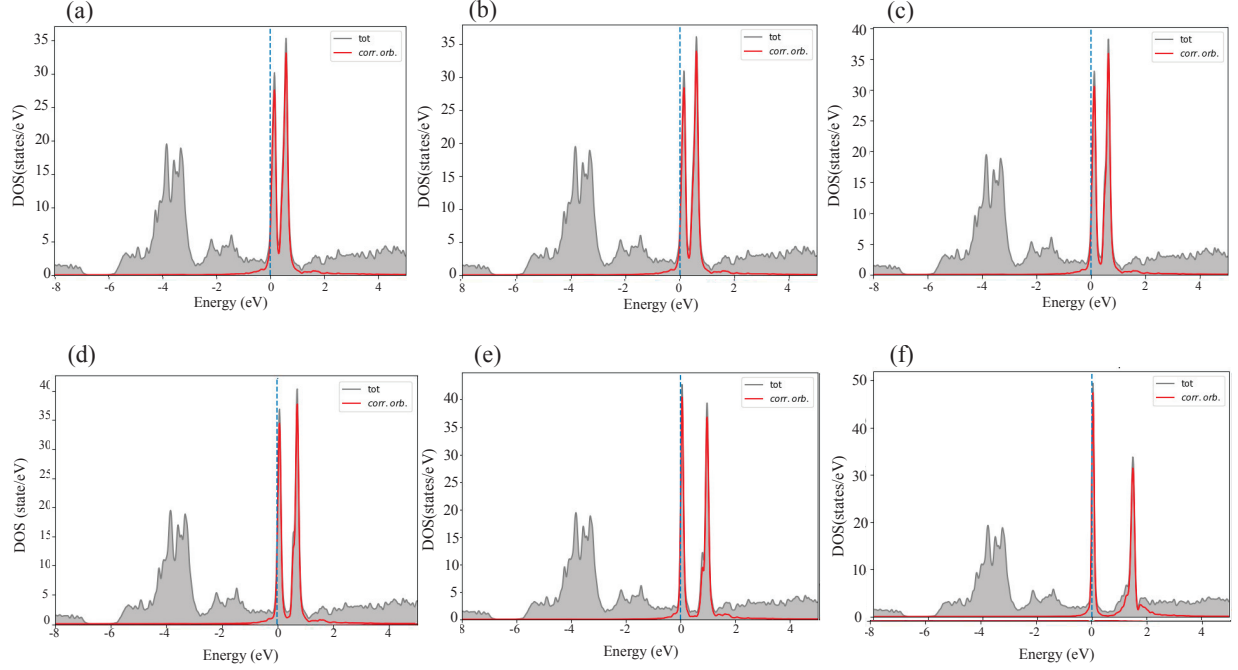

FIG. S4. **The electronic DOS for increasing  $U$**  is shown with the total DOS in black and the projected  $f$ -electron DOS in red. The values of  $U$  were tested at (a) 1eV, (b) 2eV, (c) 3eV, (d) 4eV, (e) 5eV, and (f) 6eV without taking CFS into account in the GWA calculation.

defined as

$$\Sigma_i(\omega) \equiv (I - R_i^\dagger R_i)(R_i^\dagger R_i)^{-1} \omega (R_i^{-1} \lambda_i R_i^{\dagger-1}), \quad (11)$$

where  $R$  and  $\lambda$  are block matrices in the Lagrange function implemented by Lanatà *et al.* to describe the rotationally invariant slave boson (RISB) mean-field theory [10, 11] and  $\omega$  is the fermionic Matsubara frequency.  $Z_i \equiv R_i^\dagger R_i$  are then the matrices of the quasiparticle weights. The eigenvalues of this matrix can be related to the effective mass of the quasi particle as  $1/Z = m_{qp}^*/m_e$ . These eigenvalues have been calculated with and without CFS effects and recorded in Table S1, which compares these quasiparticle weights in each case for increasing values of  $U$ . In the case where CFS is neglected, the  $f$  electrons are split into  $j = 5/2$  and  $j = 7/2$  sub-orbitals, and the magnitude of  $Z$  decreases as  $U$  increases indicating a gradual increase in the effective quasiparticle mass. The orbital occupation increases very slightly with increasing  $U$  in the  $j = 5/2$  subshell and decreases with increasing  $U$  in the  $j = 7/2$  subshell. The orbital occupations are fractional in each doublet with  $\Gamma_7^{(1)}$  having a consistently larger occupation. The

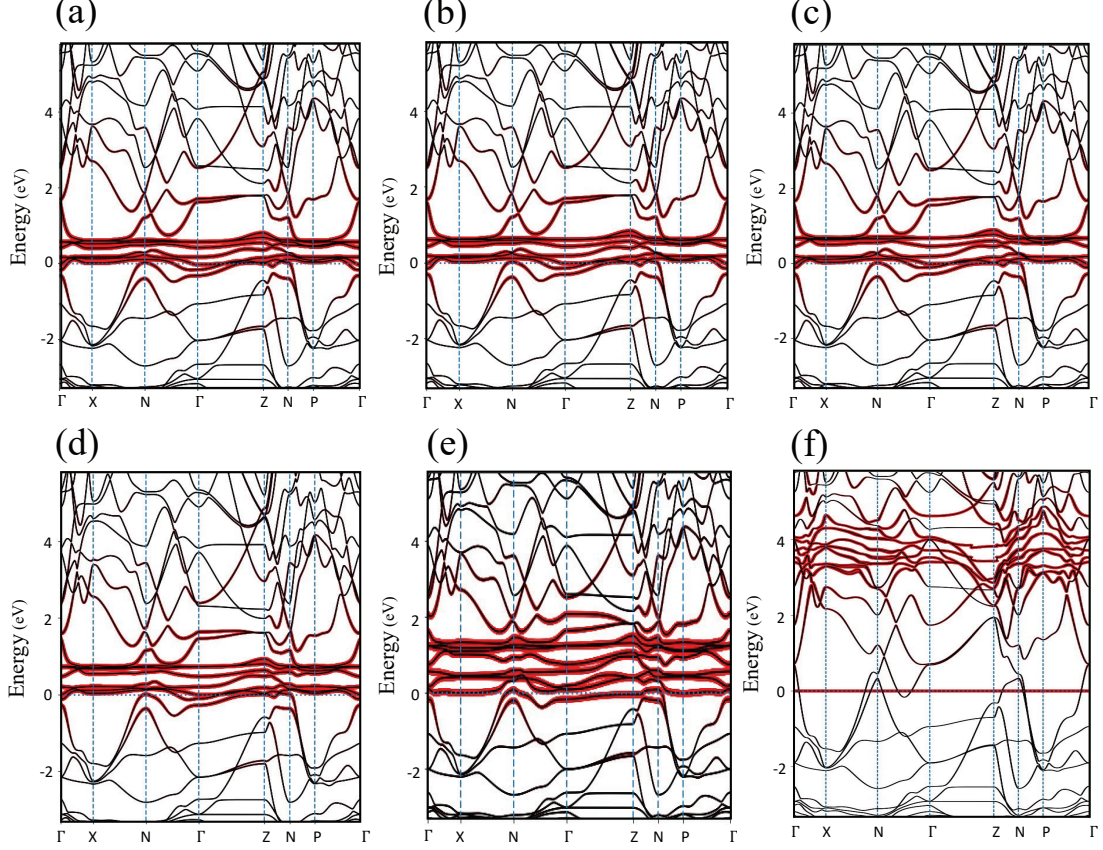

FIG. S5. **The electronic structure** for  $\text{CeCu}_2\text{Si}_2$  calculated using the GWA with CFS for increasing values of  $U$ : (a) 1eV, (b) 2eV, (c) 3eV, (d) 4eV, (e) 5eV, and (f) 6eV.  $J = 0.7\text{eV}$  for each calculation. The qualitative appearance of the band dispersions is relatively constant until  $U$  reaches a value of 5eV, at which point the  $f$ -electron bands (indicated in red) begin to spread into the higher energy conduction bands. Then at  $U = 6\text{eV}$ , the  $j = 5/2$   $f$ -electron bands flatten at the Fermi energy and the  $j = 7/2$   $f$ -electrons are shifted into the conduction bands (see FIG. S6(f)).

total occupation can be calculated by multiplying  $n$  by 2 for each Kramers doublet (e.g. for  $U=0$  with CFS,  $0.48 \times 2 + 0.02 \times 2 + 0.04 \times 2 = 1.08$ ), or in the cases without CFS it can be determined by summing the 6-fold  $5/2$  and 8-fold  $7/2$  subshells (e.g. for  $U=0$  without CFS,  $0.10 \times 6 + 0.04 \times 8 = 0.92$ ). For the calculations including CFS the relationship between  $Z$  and the Coulomb strength is non-monotonic in the excited  $\Gamma_7^{(2)}$  and  $\Gamma_6$  states. In the  $\Gamma_7^{(1)}$  Kramers doublet, defined by equation 8,  $Z$  decreases sharply between  $U = 2$  and  $U = 3\text{eV}$  and again between  $U = 5$  and  $U = 6\text{eV}$ . For the CFS calculations we have included the data point at  $U = 5.1\text{eV}$ . Here we see that

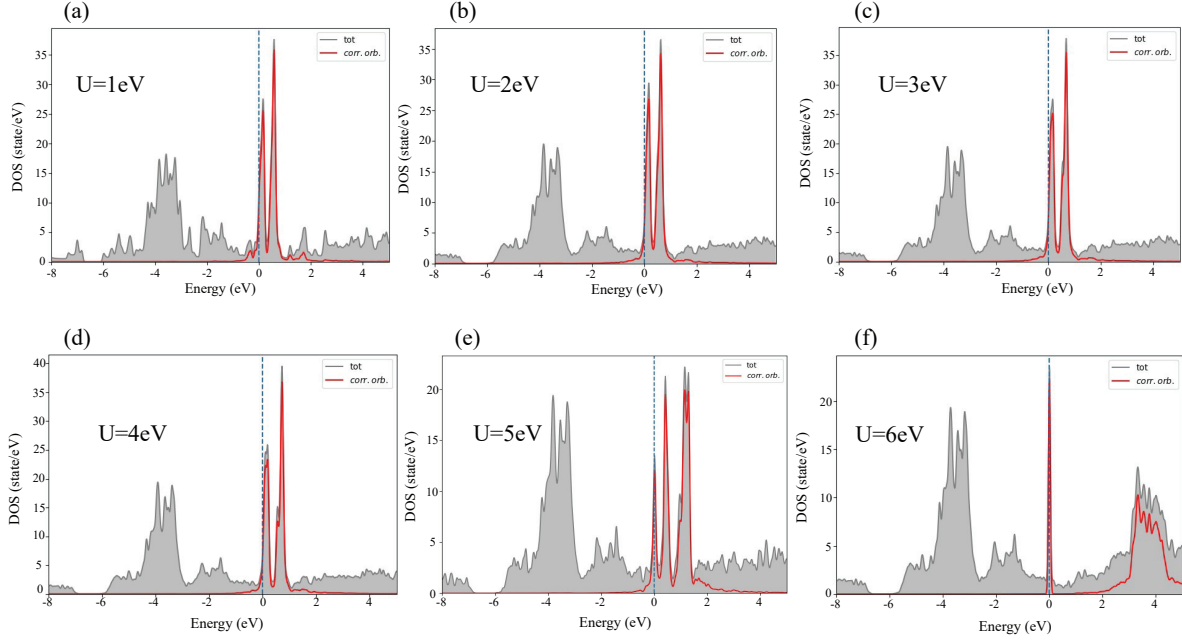

FIG. S6. **The electronic DOS for increasing  $U$**  is shown with the total DOS in black and the projected  $f$ -electron DOS in red. The values of  $U$  were tested at (a) 1eV, (b) 2eV, (c) 3eV, (d) 4eV, (e) 5eV, and (f) 6eV with CFS in the GWA.

this slight increase the the Coulomb interaction strength corresponds to a relatively sharp decrease in the quasiparticle weight in  $\Gamma_7^{(1)}$  and corresponding increase in the effective quasiparticle mass,  $m_{qp}$ . This is consistent with the evolution of the DOS and our exploration of the Fermi surface topology (see section III B), which indicates an increasingly sensitive and coupled relationship between the electronic correlations and the CFS between  $U = 5$  and 6 eV. Indeed, at  $U = 6$  eV  $Z$  approaches 0. For the  $\Gamma_7^{(2)}$  and  $\Gamma_6$  doublets, the values of  $Z$  are fairly consistent with increasing  $U$ , oscillating between  $\sim 0.96$  and  $\sim 0.8$ . The orbital occupations are fractional in each doublet with  $\Gamma_7^{(1)}$  having a consistently larger occupation. This pattern is consistent with our observations of the electronic structure's evolution in the presence of CFS and increasingly strong Coulomb interactions.

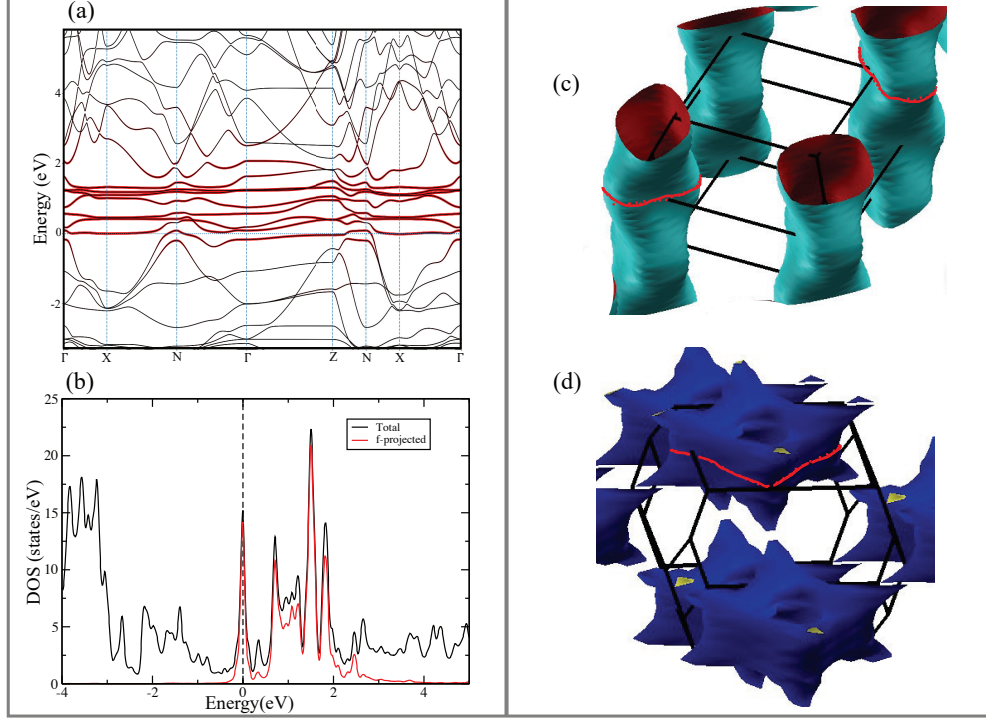

FIG. S7. **The ground state calculation for  $U = 5.1\text{eV}$**  is shown in detail. The Fermi surface sheet predicted for this value of  $U$  show the best agreement with both experimental measurements and renormalized band theory calculations.

### B. Supplementary Fermi Surface Topologies

Here we show the full Coulomb parameter analysis for the Fermi Surface of  $\text{CeCu}_2\text{Si}_2$ . The Fermi sheets calculated without CFS are shown in FIG. S8 and those calculated with CFS included are shown in FIG. S9. Additionally, we explored a DMFT approach (neglecting CFS). These Fermi surface topology results compare nearly exactly to our GWA calculation at the same value of  $U$ , which is shown in FIG. S10.

The electronic structure results from section III A are an indication that the CFS effects are significant to the renormalized band dispersion and therefor the Fermi surface. This is demonstrated by the comparison of figures S8 and S9, where FIG. S9 shows the evolution of the Fermi surface topology with increasing  $U$  with CFS included in the GWA. Here we have also included the Fermi surface at  $U = 5.1$  to demonstrate the sensitivity of these calculations in the presence of CFS. For  $U > 5$  and  $< 6\text{eV}$ , the Fermi surface topology and dHvA data becomes highly unstable, vacillating between a two-sheet Fermi surface and a single sheet as shown in section III B 1. Table S3

TABLE S1. **Eigenvalues of the  $4f$  quasiparticle matrix,  $Z$ , and corresponding orbital occupations,  $n$ ,** at  $U$  values from 0 to 6 eV. The top half of the table displays the results that include CFS effects and the bottom part of the table show results that neglect the CFS.

| With CFS    | $\Gamma_7^{(1)}$ |      | $\Gamma_7^{(2)}$ |      | $\Gamma_6$ |      |
|-------------|------------------|------|------------------|------|------------|------|
| U(eV)       | Z                | n    | Z                | n    | Z          | n    |
| 0           | 0.96             | 0.48 | 0.96             | 0.02 | 0.96       | 0.04 |
| 1           | 0.92             | 0.49 | 0.91             | 0.02 | 0.90       | 0.04 |
| 2           | 0.90             | 0.48 | 0.87             | 0.02 | 0.88       | 0.04 |
| 3           | 0.79             | 0.48 | 0.86             | 0.02 | 0.83       | 0.03 |
| 4           | 0.74             | 0.50 | 0.79             | 0.01 | 0.83       | 0.01 |
| 5           | 0.73             | 0.50 | 0.86             | 0.01 | 0.82       | 0.01 |
| 5.1         | 0.47             | 0.50 | 0.96             | 0.01 | 0.99       | 0.01 |
| 6           | 0.00             | 0.50 | 0.97             | 0.01 | 0.96       | 0.01 |
| Without CFS |                  | 5/2  | 7/2              |      |            |      |
| U(eV)       | Z                | n    | Z                | n    |            |      |
| 0           | 0.96             | 0.10 | 0.96             | 0.04 |            |      |
| 1           | 0.91             | 0.11 | 0.91             | 0.04 |            |      |
| 2           | 0.86             | 0.11 | 0.88             | 0.03 |            |      |
| 3           | 0.77             | 0.12 | 0.83             | 0.03 |            |      |
| 4           | 0.64             | 0.13 | 0.78             | 0.02 |            |      |
| 5           | 0.48             | 0.14 | 0.74             | 0.02 |            |      |
| 6           | 0.32             | 0.15 | 0.75             | 0.01 |            |      |

also shows the wide jumps in the effective cyclotron mass of the heavy band (when it is present). This may be a numerical instability in the calculations resulting in under-converged or nonphysical results. Even with very careful convergence (the  $k$ -point mesh was increased to  $17 \times 17 \times 17$  for these calculations), the  $U > 5\text{eV}$  calculations could not completely prevent the anomalous behavior. This is likely due to the complex  $4f$  electron correlations present in the heavy Fermi sheet. Not only are they sensitive to the strength of the Coulomb interactions, but the inclusion of

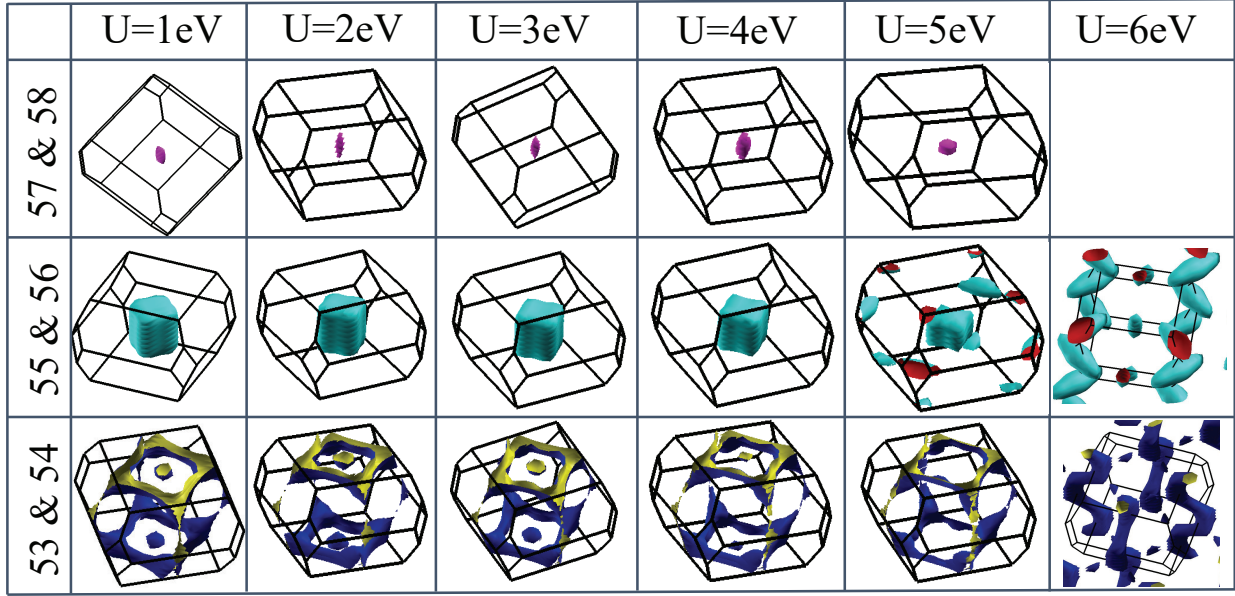

FIG. S8. **The Fermi surfaces for increasing  $U$  without CFS** are shown for degenerate bands 53 through 58. Calculations include SOC and track the evolution of the Fermi sheets as the Coulomb interaction becomes stronger.

CFS appears to make the electronic structure more volatile. Note that the absolute value of  $U$  in this case is not likely to be exactly consistent across different methods but should be viewed as an indicator of the existence of a critical point in the electronic correlation strength.

$U = 5.1\text{eV}$  is the point at which the Fermi surface topology calculated with GWA most closely agrees with experimental observation and previous theoretical studies. With CFS included there are two sheets making up the Fermi surface and the dHvA data is given in Table S2. FIG. S7 shows the electronic ground state information including the band dispersion, DOS, and Fermi sheets.

The effective mass,  $m^*$ , reported from the dHvA simulations differs from the effective quasiparticle mass,  $m_{qp}^*$ , derived from the quasiparticle weight,  $1/Z = m_{qp}^*/m_e$ . In this case  $m^*$  is the effective carrier mass averaged around an extremal cyclotron orbit (see equation 6 in the main text). This gives the instantaneous effective mass of the quasiparticles in the Fermi sheet at a particular orbit rather than the overall effective mass of the quasiparticles in the energy band. For our dHvA simulations we have calculated the cyclotron orbits for ( $\mathbf{B} \parallel z$ ). As the shape of the heavy Fermi sheet is cylindrical-like along this direction, the average effective mass is  $m^* \simeq 488$  which agrees especially well with the results from renormalized band theory[12].

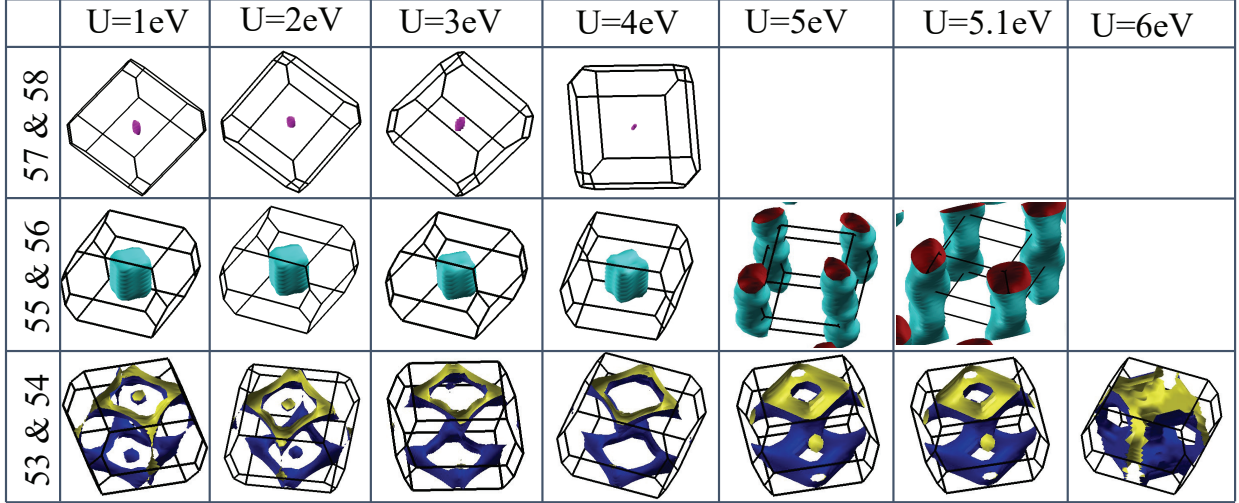

FIG. S9. **The Fermi surfaces for increasing  $U$  with CFS** are shown for degenerate bands 53 through 58. The evolution of the Fermi surface sheets shows the electronic structures sensitivity to the choice of the Hubbard Parameter,  $U$ . The calculation at  $U = 5.1\text{eV}$  is included.

### 1. Additional Fermi surface typologies

Here we present results of the GWA calculations for  $U$  from 5.1 to 5.9 eV. The Fermi surfaces and dHvA data are detailed to demonstrate the sensitivity of the  $\text{CeCu}_2\text{Si}_2$  electronic structure in the presence of strong electron-electron correlations and CFS. For these calculations the k-point grid is increased to  $17 \times 17 \times 17$  in order to mitigate any convergence related numerical problems.

We have not ruled out that this erratic dependence may be attributed to numerical anomalies in the calculations. But given very careful convergence, we are reasonably confident in the results at  $U = 5.1\text{ eV}$ . The dHvA demonstrates similar fluctuation, particularly in the effective cyclotron mass,  $m^*$ . Indeed, the ease or difficulty of the calculation does correspond to the mass renormalization. As  $m^*$  becomes very large, the simulation results tend to become less consistent, which is likely a limitation of the computational capabilities.

TABLE S2. **The dHvA and volume data for Fermi surface calculations at various U values with and without CFS.** Frequencies are given in kilotesla (kT), and corresponding effective masses are in units of electron mass ( $m_e$ ). Reciprocal occupied (electron bands 55-58) and unoccupied (hole bands 53 and 54) Fermi surface volumes are given in units of  $\text{\AA}^{-3}$ . The electron occupation,  $e^-$ , is the approximate number of electrons in the band. All measurements were taken for a magnetic field parallel to the  $z$  axis ( $\mathbf{B} \parallel z$ ). The Hubbard parameter strengths from 1 to 6 eV are compared. Band numbers are given for the odd bands in each degenerate pair.

| U(eV) | band | with CFS |        |          |       | without CFS |        |          |       |
|-------|------|----------|--------|----------|-------|-------------|--------|----------|-------|
|       |      | $f$      | $m^*$  | $V_{FS}$ | $e^-$ | $f$         | $m^*$  | $V_{FS}$ | $e^-$ |
| 0     | 53   | 10.49    | 3.282  | 0.239    | 1.840 | 10.49       | 3.282  | 0.242    | 1.838 |
|       | 55   | 3.397    | 2.480  | 0.210    | 0.141 | 3.397       | 2.480  | 0.215    | 0.144 |
|       | 57   | 0.093    | 0.884  | 0.002    | 0.001 | 0.093       | 0.884  | 0.002    | 0.001 |
| 1     | 53   | 10.46    | 4.062  | 0.230    | 1.846 | 10.36       | 3.766  | 0.231    | 1.845 |
|       | 55   | 3.162    | 2.523  | 0.187    | 0.126 | 3.243       | 2.612  | 0.193    | 0.129 |
|       | 57   | 0.229    | 1.234  | 0.006    | 0.004 | 0.171       | 1.283  | 0.004    | 0.003 |
| 2     | 53   | 10.25    | 4.067  | 0.218    | 1.854 | 10.35       | 3.937  | 0.229    | 1.846 |
|       | 55   | 3.100    | 2.559  | 0.176    | 0.118 | 3.240       | 2.707  | 0.189    | 0.127 |
|       | 57   | 0.229    | 1.338  | 0.006    | 0.004 | 0.164       | 1.422  | 0.004    | 0.003 |
| 3     | 53   | 9.799    | 5.100  | 0.191    | 1.872 | 10.27       | 4.680  | 0.220    | 1.852 |
|       | 55   | 2.963    | 2.859  | 0.150    | 0.100 | 3.172       | 3.027  | 0.173    | 0.116 |
|       | 57   | 0.234    | 1.570  | 0.006    | 0.004 | 0.205       | 1.602  | 0.005    | 0.003 |
| 4     | 53   | 9.797    | 4.283  | 0.187    | 1.874 | 10.17       | 6.491  | 0.202    | 1.865 |
|       | 55   | 2.954    | 2.600  | 0.152    | 0.102 | 3.003       | 3.947  | 0.143    | 0.096 |
|       | 57   | 0.072    | 1.240  | 0.001    | 0.001 | 0.299       | 2.114  | 0.008    | 0.005 |
| 5     | 53   | 10.71    | 4.496  | 0.382    | 1.744 | 10.35       | 9.214  | 0.203    | 1.864 |
|       | 55   | 3.854    | 26.715 | 0.356    | 0.239 | 2.741       | 72.230 | 0.149    | 0.100 |
|       | 57   | -        | -      | -        | -     | 0.357       | 3.419  | 0.005    | 0.003 |
| 5.1   | 53   | 11.45    | 4.353  | 0.518    | 1.653 | -           | -      | -        | -     |
|       | 55   | 5.910    | 488.0  | 1.007    | 0.676 | -           | -      | -        | -     |
|       | 57   | -        | -      | -        | -     | -           | -      | -        | -     |
| 6     | 53   | 18.346   | 2000   | 2.127    | 1.427 | 10.85       | 15.908 | 0.232    | 1.844 |
|       | 55   | -        | -      | -        | -     | 3.333       | 66.60  | 0.153    | 0.103 |
|       | 57   | -        | -      | -        | -     | -           | -      | -        | -     |

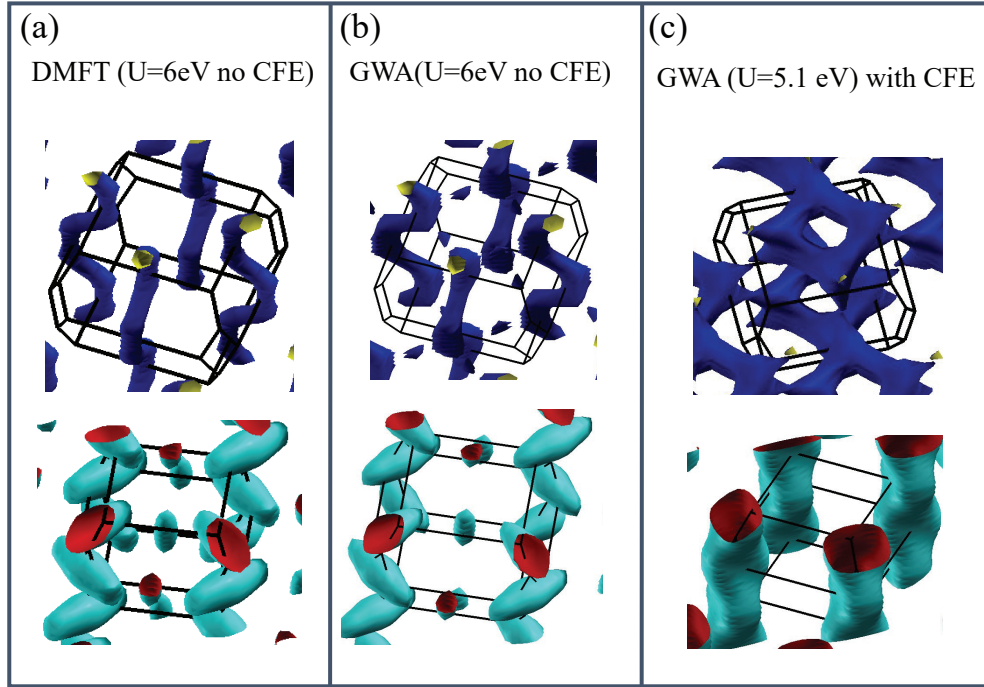

FIG. S10. **The Fermi surfaces are compared** for (a) DMFT without CFS with  $U = 6\text{eV}$ , (b) a GWA calculation without CFS at  $U = 6\text{eV}$ , and (c) a GWA calculations with CFS at  $U = 5.1\text{eV}$ . The DMFT and GWA calculations give nearly identical Fermi surface typologies. When CFS is included in the GWA method the results agree closely with experiment and renormalized band theory calculations.

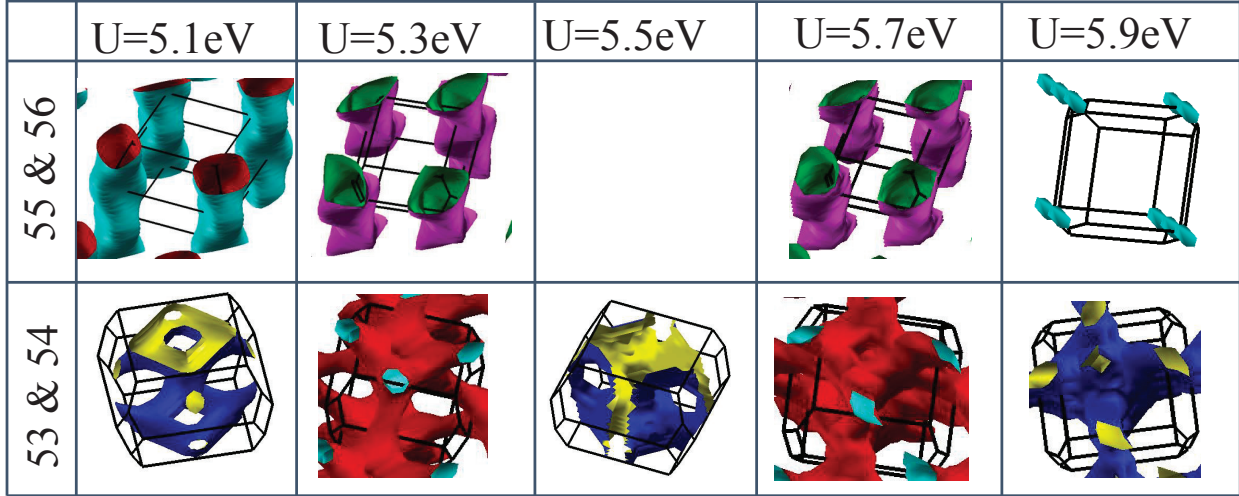

FIG. S11. **The Fermi surfaces for increasing  $U$**  are shown for degenerate bands 53 through 56. The evolution of the Fermi surface sheets shows the electronic structures sensitivity to the choice of the Hubbard parameter,  $U$ .

TABLE S3. **The dHvA and volume data for Fermi surface calculations at  $U$  values from 5.1 to 5.9 with CFS.** Frequencies are given in kilotesla (kT), and corresponding effective masses are in units of electron mass ( $m_e$ ). Reciprocal occupied (electron bands 55-56) and unoccupied (hole bands 53 and 54) Fermi surface volumes are given in units of  $\text{\AA}^{-3}$ . The electron occupation,  $e^-$ , is the approximate number of electrons in the band. All measurements were taken for a magnetic field parallel to the  $z$  axis ( $\mathbf{B} \parallel z$ ). The Hubbard parameter strengths from 5.1 to 5.9 eV are compared. Band numbers are given for the odd bands in each degenerate pair.

| U(eV) | band | $f$   | $m^*$  | $V_{FS}$ | $e^-$ |
|-------|------|-------|--------|----------|-------|
| 5.1   | 53   | 11.45 | 4.350  | 0.52     | 1.65  |
|       | 55   | 5.51  | 780.38 | 1.01     | 0.68  |
| 5.3   | 53   | 12.35 | 7.910  | 0.57     | 1.612 |
|       | 55   | 7.81  | 19.925 | 0.89     | 0.59  |
| 5.5   | 53   | 14.57 | 7.0574 | 2.12     | 1.42  |
|       | 55   | -     | -      | -        | -     |
| 5.7   | 53   | 15.15 | 11.11  | 0.85     | 1.43  |
|       | 55   | 25.16 | 155.92 | 1.05     | 0.71  |
| 5.9   | 53   | 14.91 | 8.30   | 0.89     | 1.40  |
|       | 55   | 5.86  | 149.44 | 0.99     | 0.67  |

- 
- [1] J. P. Rueff, J. M. Ablett, F. Strigari, M. Deppe, M. W. Haverkort, L. H. Tjeng, and A. Severing, *Physical Review B* **91** (2015), 10.1103/PhysRevB.91.201108.
  - [2] P. Blaha, K. Schwarz, G. K. H. Madsen, D. Kvasnicka, and J. Luitz, *WIEN2K, An Augmented Plane Wave + Local Orbitals Program for Calculating Crystal Properties* (Karlheinz Schwarz, Techn. Universität Wien, Austria, 2001).
  - [3] J.-X. Zhu, A. K. McMahan, M. D. Jones, T. Durakiewicz, J. J. Joyce, J. M. Wills, and R. C. Albers, *Phys. Rev. B* **76**, 245118 (2007).
  - [4] K. Haule, C.-H. Yee, and K. Kim, *Phys. Rev. B* **81**, 195107 (2010).
  - [5] J.-X. Zhu, M. Janoschek, R. Rosenberg, F. Ronning, J. D. Thompson, M. A. Torrez, E. D. Bauer, and C. D. Batista, *Phys. Rev. X* **4**, 021027 (2014).
  - [6] J. P. Perdew, K. Burke, and M. Ernzerhof, *Phys. Rev. Lett.* **77**, 3865 (1996).
  - [7] H. Harima and A. Yanase, *Journal of the Physical Society of Japan* **60**, 21 (1991).
  - [8] H. Harima and A. Yanase, *Journal of Magnetism and Magnetic Materials* **108**, 145 (1992).
  - [9] R.-s. Li, X. Lu, J.-t. Wang, D.-q. Xin, and X.-g. Yao, *Chinese Journal of Physics* **66**, 684 (2020).
  - [10] N. Lanatà, Y. Yao, C.-Z. Wang, K.-M. Ho, and G. Kotliar, *Physical Review X* **5** (2015), 10.1103/PhysRevX.5.011008.
  - [11] N. Lanata, Y. Yao, X. Deng, V. Dobrosavljevic, and G. Kotliar, *Phys Rev Lett* **118**, 126401 (2017), lanata, Nicola Yao, Yongxin Deng, Xiaoyu Dobrosavljevic, Vladimir Kotliar, Gabriel eng 2017/04/08 *Phys Rev Lett.* 2017 Mar 24;118(12):126401. doi: 10.1103/PhysRevLett.118.126401. Epub 2017 Mar 23.
  - [12] G. Zwicknagl, *Rep Prog Phys* **79**, 124501 (2016), zwicknagl, Gertrud eng Research Support, U.S. Gov't, Non-P.H.S. England 2016/10/25 *Rep Prog Phys.* 2016 Dec;79(12):124501. doi: 10.1088/0034-4885/79/12/124501. Epub 2016 Oct 17.
